# Supplementary material for: Dynamic Regret Analysis for Online Tracking of Time-varying Structural Equation Model Topologies
Source: arXiv:2003.08145 source file (2020-03-18)
Supplement: Supplementary file 1 [file supp.tex]

\item \cmt {Problem definition:}\\
Given: $\{\bm f[t]\}_{t=0}^{t}$

Required: $\{ \bm a_n[t]\}_{n=1}^N$   
\item \cmt{Solution:}\\
Online approach:\\

A recursive least squares (RLS) based solution for this problem is proposed here.\\
Let \\
$\bm y_n[t] := \left [ f_n[t], ~f_n[t-1],~ \ldots, ~f_n[t-L+1]\right ]^T ~\in \mathbb R^ {L}$\\ \\
$\bm F_n[t]:= 
\begin{bmatrix}
f_n[t-1] &f_n[t-2]& \ldots  &f_n[t-P] \\
f_n[t-2] &f_n[t-3]& \ldots  &f_n[t-P-1] \\
\vdots &\vdots &\ddots &\vdots \\
f_n[t-L] &f_n[t-L-1]& \ldots &f_n[t-P-L+1] 
\end{bmatrix} \in \mathbb R^ {L\times P}$\\ \\ \\
$\bm F[t]:=\left [ \bm F_1[t], ~ \bm F_2[t],~ ..., ~ \bm F_{N}[t]\right ]~~\in \mathbb R^ {L\times PN}$\\ \\ 
$\bm a_{n,n'}[t]:=[a_{n,n'}^{(1)}[t], ~ a_{n,n'}^{(2)}[t],~ ..., ~a_{n,n'}^{(P)}[t]^T ~~\in \mathbb R^ {P}$\\

$\bm a_{n}[t]:=[\bm a_{n,1}[t], ~ \bm a_{n,2}[t], ~ ..., ~\bm a_{n,N}[t]]^T ~~ \in \mathbb R^ {PN}$\\ \\
Sliding Window Regularized RLS:\\
Consider least squared error
\begin{align}
 \mathcal{E}_L^{(n)}[t]&= \left \lVert \bm y_n[t]- \bm F[t] \bm a_n[t] \right \lVert_2 \\
 &=\sum_{\tau=t-L+1}^{t}\left \lvert f_n[\tau]- \bm F_{t-\tau +1:}[t]\bm a_n[t] \right \lvert^2.
 \end{align}
The $(t-\tau +1)$-th row of $\bm F[t]$ can be represented as $\bm g_{t-\tau +1}^T[t]$, so 
 \begin{align} 
   \mathcal{E}_L^{(n)}[t]&=\sum_{\tau=t-L+1}^{t}\left \lvert f_n[\tau]- \bm g_{t-\tau +1}^T[t]\bm a_n[t] \right \lvert^2\\
 &=\sum_{\tau=t-L+1}^{t}\left \lvert e[\tau] \right \lvert^2.
\end{align}
The overall estimation criterion for regularized sliding window RLS  is
\begin{align}
 \hat{\bm a}_n^{\text{RLS}}[t]&=\underset{\bm a_n[t]}{\arg\min} ~~ \mathcal{E}_L^{(n)}[t]+\lambda \sum_{n'=0}^{N} \left \lVert \bm a_{n,n'}[t]\right\rVert_2\\
&=\underset{\bm a_n[t]}{\arg\min} ~~ \sum_{\tau=t-L+1}^{t}\left \lvert f_n[\tau]- \bm g_{t-\tau +1}^T[t]\bm a_n[t] \right \lvert^2+\lambda \sum_{n'=0}^{N} \left \lVert \bm a_{n,m}[t]\right\rVert_2
\end{align}

\end{itemize}
